# Supplementary material for: Probing Patchy Saturation of Fluids in Nanoporous Media by Ultrasound
Source: arXiv:1802.06262 source file (2018-02-17)
Supplement: Supplementary file 1 [file SM-saturation.pdf]

# Probing Patchy Saturation of Fluids in Nanoporous Media by Ultrasound
# Supplementary Material

Boris Gurevich,[1,2] Michel M. Nzikou,[1] and Gennady Y. Gor[3]

[1] *Curtin University, Perth, Western Australia, Australia*

[2] *CSIRO, Perth, Western Australia, Australia.*

[3] *Department of Chemical, Biological and Pharmaceutical Engineering*

*New Jersey Institute of Technology, Newark, NJ, USA*

## SM.1. CONCENTRIC SPHERE PATCHY SATURATION MODEL

Johnson [1] derived a general approximate solution for the complex-valued bulk modulus $K_{sat}$ of a poroelastic medium consisting of regions (patches) saturated with fluids 1 and 2, [1, Eq. 43]

$$K_{sat} = K_{GH} - \frac{K_{GH} - K_{GW}}{1 - \zeta + \zeta\sqrt{1 - i\omega\tau\zeta^2}}, \tag{SM.1}$$

where $K_{GW}$ and $K_{GH}$ are Gassmann-Wood and Gassmann-Hill limits defined in the main text, $\omega$ is angular frequency, while $\tau$ and $\zeta$ are time-scale parameters defined by [1, Eq. 44]

$$\tau = \left(\frac{K_{GH} - K_{GW}}{K_{GH}\mathcal{G}}\right)^2, \tag{SM.2}$$

and [1, Eq. 45]

$$\zeta = \frac{K_{GH} - K_{GW}}{2K_{GW}}\frac{\tau}{\mathcal{T}}. \tag{SM.3}$$

Parameters $\mathcal{T}$ and $\mathcal{G}$ describe asymptotic behaviour of attenuation at low and high frequencies and are controlled by the geometry of the patches. Parameter $\mathcal{G}$ in Eq. SM.2 is given by [1, Eqs. 34, 37]:

$$\mathcal{G} = \frac{S}{\phi V}\frac{\kappa K_{GH}}{\eta_1\sqrt{D_1} + \eta_2\sqrt{D_2}}\frac{(R_2 + Q_2)/M_G^{(2)} - (R_1 + Q_1)/M_G^{(1)}}{S_2K_G^{(2)}/M_G^{(2)} + S_1K_G^{(1)}/M_G^{(1)}}, \tag{SM.4}$$

where $S/V$ is the surface to volume ratio for the patches, $M_G^{(1,2)} = K_G^{(1,2)} + (4/3)G_0$, and [1, Eq. 8]

$$D_{1,2} = \frac{\kappa}{\phi^2\eta_{1,2}}\frac{P_{1,2}R_{1,2} - Q_{1,2}^2}{P_{1,2} + 2Q_{1,2} + R_{1,2}} \tag{SM.5}$$

with [1, Eq. 5]

$$P_{1,2} = \frac{(1-\phi)\left(1 - \phi - K_0/K_s\right)K_s + \phi(K_s/K_{f1,2})K_0}{1 - \phi - K_0/K_s + \phi K_s/K_{f1,2}} + \frac{4}{3}G_0, \tag{SM.6}$$

$$Q_{1,2} = \frac{\left(1 - \phi - K_0/K_s\right)\phi K_s}{1 - \phi - K_0/K_s + \phi K_s/K_{f1,2}}, \tag{SM.7}$$

and

$$R_{1,2} = \frac{\phi^2 K_s}{1 - \phi - K_0/K_s + \phi K_s/K_{f1,2}}. \tag{SM.8}$$

The simplest patch geometry is that of a double spherical shell, where the inner sphere of radius $R_i$ is saturated with fluid 2 and is surrounded by an outer sphere with radius $R_o$,

with the region between the two spheres saturated with fluid 1, so that $S_2 = (R_i/R_o)^3$. For this case the expression for $\mathcal{T}$ reads [1, Eq. 40]

$$\mathcal{T} = \frac{\phi^2 K_{GW}}{30\kappa R_o^3} \left\{ \left[3\eta_2 g_2^2 + 5(\eta_1 - \eta_2) g_1 g_2 - 3\eta_1 g_1^2\right] R_i^5 \right.$$
$$-15\eta_2 g_2 (g_2 - g_1) R_i^3 R_o^2 +$$
$$\left. 5 g_2 \left[3\eta_2 g_2 - (2\eta_2 + \eta_1) g_1\right] R_i^2 R_o^3 - 3\eta_2 g_2^2 R_o^5 \right\} \quad \text{(SM.9)}$$

with [1, Eq. 20]

$$g_{1,2} = \frac{\left(1 - \frac{K_0}{K_s}\right)\left(\frac{1}{K_{GW}} - \frac{1}{K_{f1,2}}\right)}{1 - \frac{K_0}{K_s} - \frac{\phi K_0}{K_s} + \frac{\phi K_0}{K_{GW}}}. \quad \text{(SM.10)}$$

## SM.2. MODELING PARAMETERS

For the samples used in the sorption experiments [2, 3], the parameters of the Vycor glass and fluids are given in Tables SM.1 and SM.2. Bulk modulus, $K_0$, shear modulus $G_0$, and porosity $\phi$ of the dry Vycor glass were reported in [2, 3].

Page et al. [2] also give a measured density of the dry Vycor glass: $\rho_0 = 1.54$ g cm$^3$. From this value, the density of the solid glass is obtained as $\rho_s = \rho_0/(1-\phi) = 2.229$. We use this value of solid density for modelling both experiments.

Permeability of Vycor was measured by Vichit-Vadakan and Scherer [4]. The solid Vycor "backbone" modulus cannot be measured directly and varies from sample to sample [5, 6]. For this study we used the values inverted with an elastic effective medium theory [6].

The density of argon was taken from [7], density of n-hexane was taken from [2]. Viscosity of liquid argon at 85 K: $\eta = 2.778 \times 10^{-4}$ Pa s, Table 14 from [8], viscosity of argon vapor at 90 K, at 0.1 MPa: $\eta = 7.46 \times 10^{-6}$ Pa s, Table 21 from [8]. Viscosity of liquid n-hexane $\eta = 0.3 \times 10^{-3}$ Pa s, taken from [2], which is close to the reference data in [9]. Viscosity of n-hexane vapor at normal pressure at 290 K is $\eta \simeq 6 \times 10^{-6}$ Pa s, Figures 1 and 3 in [9]. The adiabatic bulk modulus for argon at $T = 80$ K was taken $K_\mathrm{f} = 1.06$ GPa [10]. Bulk argon freezes at $T = 83.81$ K, and can stay liquid at $T = 80$ K only when confined; therefore the properties for liquid argon are taken at saturation at higher temperatures and extrapolated to $T = 80$ K [11]. For n-hexane at $T = 295.75$ K at saturation we take $K_\mathrm{f} = 0.803$ GPa, following [2]; this value is consistent with the more recent high-quality measurements [12]. Note that the vapor properties (density, viscosity and bulk modulus) are vanishingly small compared with the values in the liquid state and don't affect the result of the modeling.

| Ref. | $K_0$ | $G_0$ | $K_s$ | $\rho_s$ | $\phi$ | $\kappa$ |
|---|---|---|---|---|---|---|
| | GPa | GPa | GPa | g cm$^{-3}$ | | m$^2$ |
| [2] | 10.1 | 6.86 | 24 | 2.229 | 0.309 | $6 \times 10^{-20}$ |
| [3] | 7.73 | 6.86 | 16.2 | 2.229 | 0.28 | $6 \times 10^{-20}$ |

TABLE SM.1. Properties of the Vycor glass samples

| Fluid | $\rho_{f2}$ | $\eta_2$ | $K_{f2}$ |
|---|---|---|---|
| | g cm$^{-3}$ | Pa s | GPa |
| n-Hexane | 0.66 | $3 \times 10^{-4}$ | 0.803 |
| Argon | 1.4 | $2.7 \times 10^{-4}$ | 1.06 |

TABLE SM.2. Properties of the adsorbates

## SM.3. FINITE ELEMENT SIMULATIONS

As discussed in the main text, the most likely explanation for the observed saturation dependency of the modulus, velocity and attenuation on desorption is that the desorption occurs progressively from the surface of the cylindrical sample. That is, when the vapor pressure is reduced below the capillary condensation point, the Vycor sample of radius $r$ consists of a fully saturated ($S_l = 1$) inner cylindrical core of radius $r_i$ and the outer cylindrical shell with $S_l = S_{l0} = 0.4$, where

$$r_i = S_1^{1/2} r \tag{SM.11}$$

and, as before

$$S_1 = (S_l - S_{l0})(1 - S_{l0}), \tag{SM.12}$$

see Fig. SM.1.

To test this interpretation, we conduct numerical simulations of elastic wave propagation in such a configuration using ABAQUS/Explicit finite element software [13]. The two cylindrical regions are assumed to be elastic with the shear modulus of the dry sample and bulk modulus given by the Gassmann-Wood model (equations (1) and (3)). To replicate the experiment of [2], the source and receiver transducers of the same radius as the sample are attached to the opposite faces of the cylindrical sample. The source transducer emits a sinusoidal displacement pulse of the total duration of 3$\mu$s and frequency of 6.2 MHz. This

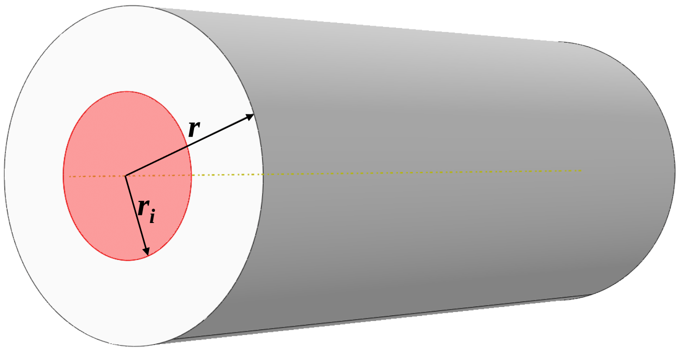


FIG. SM.1. Finite element simulation design. Area painted red (of radius $r_i$) is the fully saturated core, while the white part has saturation $S_l = S_{l0} = 0.4$

is repeated for a range of values of $r_i$ as given by equations (SM.11) and (SM.12), where liquid n-Hexane saturation $S_l$ varied from $S_l = S_{l0}$ to $S_l = 1$. The recorded wave forms are shown in Fig. SM.2.

These wave forms were used to estimate the ultrasonic velocities and attenuation factors. Velocity of the trace for $S_l = 1$ was obtained by picking the travel time manually. Then for each other trace, the travel time lag was obtained by cross-correlation with the first trace. Attenuation was calculated from amplitudes obtained by averaging a number of peaks. The modulus, velocity and attenuation computed from the simulations are shown in Figures 3a, 5a and 4, respectively, and show excellent agreement with the measurements.

[1] D. L. Johnson, J. Acoust. Soc. Am. **110**, 682 (2001).

[2] J. H. Page, J. Liu, B. Abeles, E. Herbolzheimer, H. W. Deckman, and D. A. Weitz, Phys. Rev. E **52**, 2763 (1995).

[3] K. Schappert and R. Pelster, Europhys. Lett. **105**, 56001 (2014).

[4] W. Vichit-Vadakan and G. W. Scherer, J. Am. Ceram. Soc. **83**, 2240 (2000).

[5] D. P. Bentz, E. J. Garboczi, and D. A. Quenard, Modell. Simul. Mater. Sci. Eng. **6**, 211 (1998).

[6] G. Y. Gor and B. Gurevich, Geophys. Res. Lett. **45**, 146 (2018).

[7] C. Tegeler, R. Span, and W. Wagner, J. Phys. Chem. Ref. Data **28**, 779 (1999).

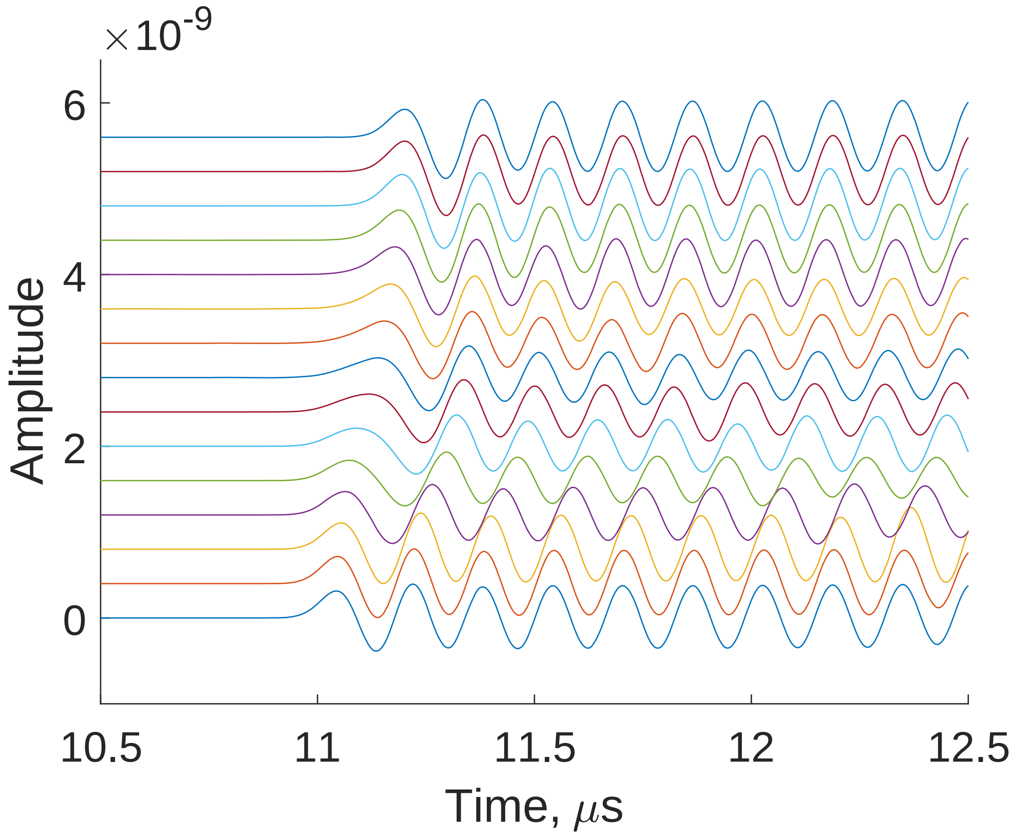


FIG. SM.2. Simulated displacement waveform for a cylindrical sample. From top to bottom trace, the inner saturated core radius $r_i$ increases from 0.01mm ($S_1 \approx 0$, $S_l \approx S_{l0} = 0.4$) to 3.5 mm ($S_1 = S_l = 1$) .

[8] H. J. Hanley, R. D. McCarty, and W. M. Haynes, J. Phys. Chem. Ref. Data **3**, 979 (1974).

[9] R. A. Perkins, M. L. Huber, M. J. Assael, E. K. Mihailidou, S. K. Mylona, and E. A. Sykioti, Pure Appl. Chem. **87**, 321 (2015).

[10] G. Y. Gor, D. W. Siderius, C. J. Rasmussen, W. P. Krekelberg, V. K. Shen, and N. Bernstein, J. Chem. Phys. **143**, 194506 (2015).

[11] G. Y. Gor, Langmuir **30**, 13564 (2014).

[12] J. L. Daridon, B. Lagourette, and J.-P. E. Grolier, Int. J. Thermophys. **19**, 145 (1998).

[13] *Abaqus 2017*, Dassault Systèmes, Providence, RI (2016), URL `https://www.3ds.com/products-services/simulia/`.
